# Supplementary material for: Learning Aerial Image Segmentation from Online Maps
Source: arXiv:1707.06879 source file (2017-07-21)
Supplement: Supplementary file 1 [file appendix.tex]

{
\begin{table}
	\tiny
	\begin{center}
    		\begin{tabular}{| l | l | l | l |}
	    		\hline
	    		Parameter layer & No. of filters & Filter sizes & No. of bias parameters \\ \hline
			conv\textunderscore 1\textunderscore 1 & 64 & (3, 3, 3) & 64 \\ \hline
			conv\textunderscore 1\textunderscore 2 & 64 & (64, 3, 3) & 64 \\ \hline
			conv\textunderscore 2\textunderscore 1 & 128 & (64, 3, 3) & 128 \\ \hline
			conv\textunderscore 2\textunderscore 2 & 128 & (128, 3, 3) & 128 \\ \hline
			conv\textunderscore 3\textunderscore 1 & 256 & (128, 3, 3) & 256 \\ \hline
			conv\textunderscore 3\textunderscore 2 & 256 & (256, 3, 3) & 256 \\ \hline
			conv\textunderscore 3\textunderscore 3 & 256 & (256, 3, 3) & 256 \\ \hline
			conv\textunderscore 4\textunderscore 1 & 512 & (256, 3, 3) & 512 \\ \hline
			conv\textunderscore 4\textunderscore 2 & 512 & (512, 3, 3) & 512 \\ \hline
			conv\textunderscore 4\textunderscore 3 & 512 & (512, 3, 3) & 512 \\ \hline
			conv\textunderscore 5\textunderscore 1 & 512 & (512, 3, 3) & 512 \\ \hline
			conv\textunderscore 5\textunderscore 2 & 512 & (512, 3, 3) & 512 \\ \hline
			conv\textunderscore 5\textunderscore 3 & 512 & (512, 3, 3) & 512 \\ \hline
			conv\textunderscore 6 & 4096 & (512, 7, 7) & 4096 \\ \hline
			conv\textunderscore 7 & 4096 & (4096, 1, 1) & 4096 \\ \hline
			conv\textunderscore 11 & 3 & (4096, 1, 1) & 3 \\ \hline
			deconv\textunderscore 1 & 3 & (3, 4, 4) & - \\ \hline
			conv\textunderscore 10 & 3 & (512, 1, 1) & 3 \\ \hline
			deconv\textunderscore 2 & 3 & (3, 4, 4) & - \\ \hline
			conv\textunderscore 9 & 3 & (256, 1, 1) & 3 \\ \hline
			deconv\textunderscore 3 & 3 & (3, 4, 4) & - \\ \hline
			conv\textunderscore 8 & 3 & (128, 1, 1) & 3 \\ \hline
			deconv\textunderscore 4 & 3 & (3, 8, 8) & - \\ \hline
		\end{tabular}
	\end{center}
	\caption{Learnable parameters of FCN-4s-1. Learnable parameters are contained in convolutional layers and deconvolutional layers. The second column of the table indicates the number of filters of each layer. The number of filters corresponds to the number of feature channels (\(D\)), which each layer outputs. The third column indicates the filter sizes (\(D' \times h \times w\)) of each layer. \(D'\) is the number of input feature channels and \(h \times w\) is the two-dimensional, spatial dimensions of the filters. The total number of learnable parameters in FCN-4s-1 is $134276540$.}
	\label{tab:shape_of_parameter_layers_FCN-4s-1}
\end{table}
